# Supplementary material for: VP-NTK: Exploring the Benefits of Visual Prompting in Differentially Private Data Synthesis
Source: arXiv:2503.16195 source file (2025-03-20)
Supplement: Supplementary file 1 [file appendix.tex]

% \section{Appendix}
% \label{sec: Appendix}

% \subsection{Proof of Theorem}
% \textit{Proof}: The DP-NTK framework consists of two key phases: model pre-training and differentially private (DP) training. In the pre-training phase, extra public data is used to train a conditional GAN. The public data is chosen to have the same number of classes as the private data but remains independent of the private dataset, resulting in zero privacy cost during this phase. After pre-training, only the generator and the feature extractor, which includes the early layers of the discriminator, are retained and frozen for the next phase. In the DP training phase, private data is processed using a pre-defined label mapping, the pre-trained generator, and the feature extractor to calculate the mean embedding $\hat{\mu}_P$. To ensure differential privacy, noise is injected into the mean embedding using the Gaussian mechanism\cite{dwork2014algorithmic}, producing $\tilde{\mu}_P = \hat{\mu}_P + \mathcal{N}(0, \frac{4\sigma^{2}}{m^{2}}I)$, where $\frac{2}{m}$ is following the result of \cite{harder2021dpmerf} and $\sigma\geq \sqrt{2\log(1.25/\delta)}/\epsilon$ is following \cite{dwork2014algorithmic}. Such the step incurs a privacy cost of $(\epsilon, \delta)$. This noisy embedding is the only part that requires privacy preservation. The framework then randomly generates Gaussian noise and labels to calculate the mean embedding iteratively, compute the loss against $\tilde{\mu}_P$, and update the visual prompting, a noise component that incurs no additional privacy cost due to the post-processing property of differential privacy. 
